# Supplementary material for: Deep Extrapolation for Attribute-Enhanced Generation
Source: arXiv:2107.02968 source file (2021-10-25)
Supplement: Supplementary file 1 [file supplement.tex]

\begin{document}

\end{document}
